# Supplementary material for: Leaky Cauldron on the Dark Land: Understanding Memory Side-Channel Hazards in SGX
Source: arXiv:1705.07289 source file (2017-08-30)
Supplement: Supplementary file 1 [file appendix.tex]

\ignore{
\section{Example Codes}
\label{app:timing}
\begin{figure}
\centering
\begin{lstlisting}
int sum(int n) {
  int ret = 0;
  if(n > 0) {
   for( int i = 0; i < n; i++)
	 ret += i;
  } else {
	 ...
  }
  return ret;
}
\end{lstlisting}
\caption{An example of secret-dependent branch leaking timing information.}\label{lst:timing}
\end{figure}
}

\section{Single-page T-SPM attack on bloom filter} 
As mentioned earlier, our study shows that the T-SPM attack even works when the
whole enclave program is on a single page, which does not expose \textit{any}
input-dependent page-access trace through the page-fault attack, since
consecutive visits to the same page cannot be observed from page faults.
However, the operations within the page could still be observed from the
execution time measured between two reference points\ignore{ monitored through
their A bits}.  Specifically, we converted a common implementation of Bloom
filter~\cite{github.bloom} into an SGX version, which reads outside enclave an integer to check its membership. In our experiment, the whole program was placed on a single
memory page in enclave. The enclave also contains an exit page automatically visited by
\texttt{XSAVE} to save the processor state when enclave exits.
%The program therefore contains two pages, with an exit page automatically
%visited by \texttt{XSAVE} to save the processor state.
This Bloom filter runs 10 hash functions one by one to check the presence of an
integer in its array: each function reports an array position and if it is zero,
then the integer is considered not a member of the array; otherwise (i.e., all
positions, as output by the all 10 functions, are set to one), the integer is
considered to be a member.

\begin{figure}
\centering
\includegraphics[width=\columnwidth]{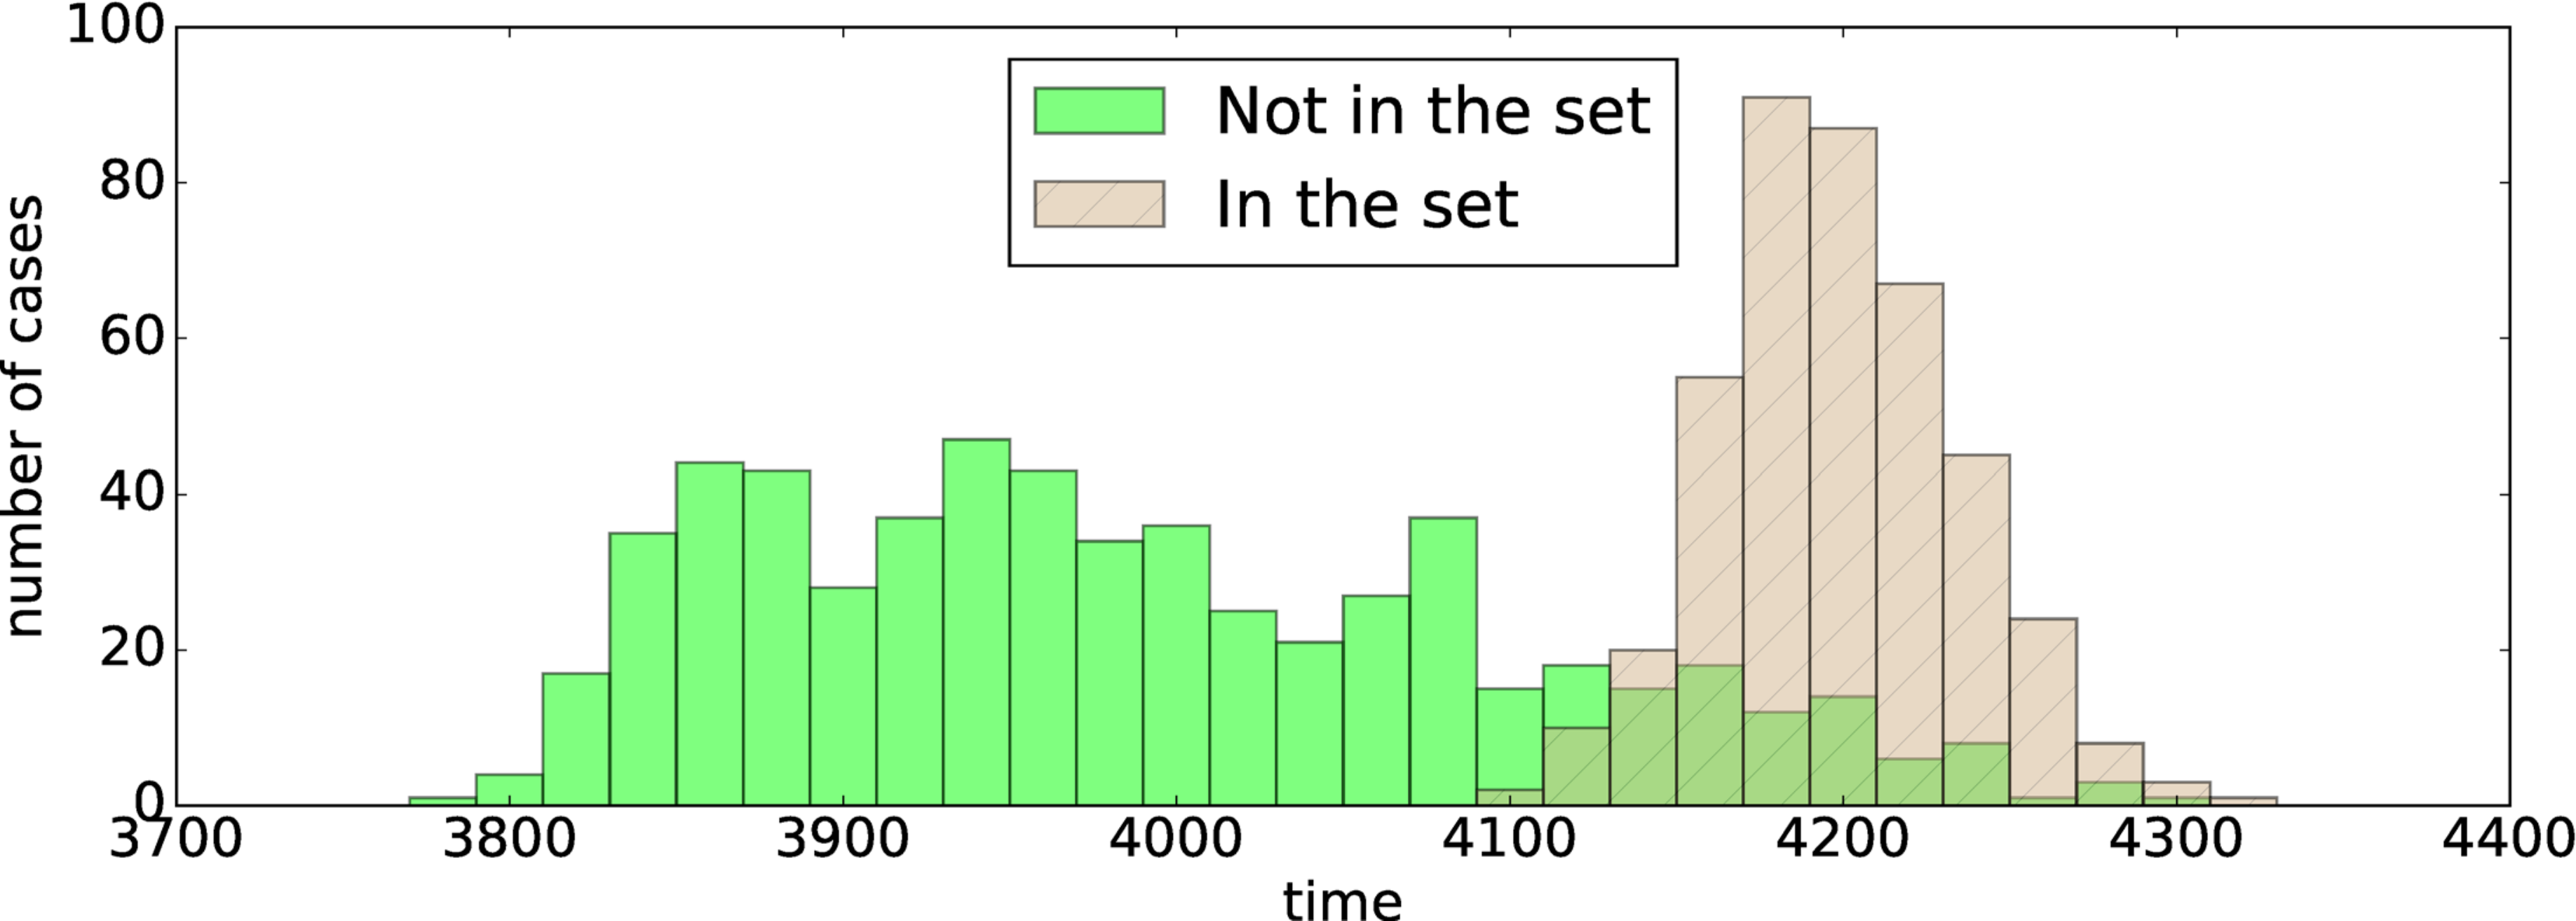}
\caption{Bloom Filter: observed time for elements in or not in the set.}
\label{fig:bf}
\end{figure}

This membership test clearly leaks out timing information, particulary for the
integers not inside the array and captured by the first a few hash operations.
In this case, the execution is shorter than that on the members, which forces
every hash function to be run on the integer.  In our experiment, we set those
two pages as references and utilized an attack process to monitor when the exit
page was visited, indicating the end of a query. At that point, the attacker
recorded the time for a query. In our experiment, we continuously queried the
Bloom filter for 1000 integers. For each integer we recorded the average time
over 100 queries. Table~\ref{fig:bf} illustrates the distribution over execution
time. The attack process inspected the page tables at the rate of once per 132
cycles, and was capable of catching 88.64\% of non-members at a precision of
95.44\%, and 93.95\% of members with a precision of 85.84\%, using a threshold
of 4143 cycles. We observed no performance impact caused by the attack. The
attack shows that same page protection may not be an effective solution to the
information leaks through page tables.

%%-----------------------------------------------

\ignore{
\section{T-SPM attack on Freetype 2.5.3}
\label{appendix:freetype}
\begin{table}
\centering
{\footnotesize
\begin{tabular}{m{0.6in}<{\centering}|m{1.2in}<{\centering}}
\Xhline{1pt}
trigger page & 0x0005B000\\
\hline
\multirow{5}{*}{\textbf{$\alpha$-$\beta$ pairs}} & 0005B000, 0005B000   \\
& 0005B000, 00065000  \\
& 0005B000, 0005E000 \\
& 00065000, 00022000 \\ 
& 0005E000, 00018000 \\
\Xhline{1pt}
\end{tabular}
\caption{Features used in Freetype experiment.}
\label{table:freetypefeature}
}
\end{table}

\begin{table}
\centering
{\footnotesize
\begin{tabular}{c|c|c|c|c|c}
\Xhline{1pt} %\\
\textbf{coverage} & 100\% & 88.17\% & 75.62\% & 69.14\% & 57.35\% \\ \Xhline{0.5pt}
\textbf{precision} & 69.90\% & 75.25\% & 80.66\% & 84.45\% & 89.94\% \\
\Xhline{1pt}
\end{tabular}
\caption{T-SPM attack on Freetype 2.5.3: for example, we achieved a precision of 69.90\% over a coverage of 100\% characters.}\label{table:freetype}
}
\end{table}
}
